# Supplementary material for: The Study of a Fibre Z-Pinch
Source: arXiv:physics/0703207 source file (2007-03-23)
Supplement: Supplementary file 1 [file appendixA.tex]

\appendix

\section{Applied spectroscopic methods}
The basic theory of emission spectroscopy will be introduced in
this section so as we could describe the spectroscopic methods. As
there are numerous spectroscopic methods \cite{Griem64, Griem74,
Hauer91, Griem97, Thorne99} we will deal only with those that were
used in our experiment.

\section{Introduction}
The characteristic property of plasma is its radiating in a
broadband spectral region. Therefore emission spectroscopy is a
diagnostic technique that has been applied to an evaluation of
appropriate plasma parameters since the very beginning of plasma
physics \cite{Griem64,deMichelis81}. By emission spectroscopy it
is possible to measure
 plasma composition,  electron temperature and density,
 ion temperature and density, electric and magnetic
field, plasma motion or turbulence, plasma dynamics, ionization
dynamics, etc~\cite{Kunze89}. The measurement of these quantities
is possible provided that transition probabilities (i.e.
oscillator strengths), and collision cross--sections are
known\footnote{On the contrary to that if we determine plasma
parameters by other non--spectroscopic methods, e.g. by laser
interferometry and laser scattering, we can experimentally measure
or verify transition probabilities or collision cross--sections.
This experimental measurement is still needed~\cite{Kunze02}.}.

As the temperature of $Z$--pinches varies from several eVs up to
tens of keV, a predominant fraction of the electromagnetic
radiation is emitted in XUV and X--ray spectral region. The
boundaries of XUV and X--ray ranges are not all rigid, but are
those traditionally accepted in the fields of X--ray spectroscopy,
plasma physics, astrophysics, X--ray laser etc. For the purpose of
this paper, we used the following wavelength ranges~\cite{Pikuz01}

\begin{figure}
\center{
\begin{tabular}{|l|l|}
\hline \hline Spectral region& Wavelength  \\
\hline
X--ray & 0.01~nm $\div$ 2.5 nm \\
\hline
hard X--ray & 0.01~nm $\div$ 0.2 nm \\
\hline
soft X--ray & 0.2~nm $\div$ 2.5 nm \\
\hline
XUV & 2.5~nm $\div$ 40 nm \\
\hline
VUV & 40~nm $\div$ 200 nm \\
\hline\hline
\end{tabular}
\caption{Definition of wavelength ranges used in our work.}}
\end{figure}

\section{Radiative processes}
Radiative processes in a plasma can be divided into three main
groups according to the type of transition. We can distinguish
transitions between two states of electrons -- free and bound.
\begin{itemize}
\item \emph{Free--free transitions} are associated with a gain or
loss of an electron energy in the field of an
ion\footnote{Collision between two electrons cannot produce
radiation by electric or magnetic dipole processes.}.  As free
states are not quantized therefore a broad continuum radiation is
created. At long wavelengths, the free--free emission approaches
the blackbody function. The loss of the electron energy into the
radiation is connected with the deceleration of electrons and
therefore we speak about Bremsstrahlung radiation. The absorption
of a photon by an electron is called as the inverse
Bremsstrahlung.

\item \emph{Free--bound transitions} correspond to the
recombination and photoionization processes. Recombination
continuum extends from each bound state of an electron and is
characterized by edges. Similarly, the absorption edges occur in
the spectral dependence of the photoionization cross--section.

\item \emph{Bound--bound transitions} occur when an electron
bounded by an ion makes a transition to another bound state. When
the final state has lower energy than the initial one, the photon
of well--defined energy is emitted. The inverse mechanism is the
photoexcitation. The radiation is characterized by emission or
absorption spectral lines.

The rate of spontaneous emission from the upper energy level ``u''
to lower level ``l'' is defined by means of Einstein probability
coefficient $A_\mathrm{ul}$ as follows
\begin{equation}
\frac{\diff n_\mathrm{u}}{\diff t}\Bigg|_{\mathrm{u}\rightarrow
\mathrm{l}}=-A_\mathrm{{ul}} n_\mathrm{u}
\end{equation}

where $n_\mathrm{u}$ is the number density of electrons in the
upper level. The overall rate of spontaneous radiative transition
from the upper level ``u'' is given by the sum of the rates from
the upper level ``u'' to all lower levels
\begin{equation}
\frac{\diff n_\mathrm{u}}{\diff
t}=-\sum_{\mathrm{l}<\mathrm{u}}A_\mathrm{{ul}}
n_\mathrm{u}=-A_\mathrm{u\rightarrow} n_\mathrm{u}
\end{equation}

The probability of spontaneous emission $A_\mathrm{ul}$ is treated
in quantum electrodynamics and is given by a selection rules. As
far as our experiments with carbon fibres are concerned, we
observed only allowed transitions with $\langle
l|e\vec{r}|u\rangle\neq 0$. The transitions that can occur by
magnetic dipole and electric quadrupole were very weak since the
plasma density was not sufficiently low. The intercombination
lines with $\triangle \mathbb{S}\neq 0$ are not usually observed
for low--$Z$ elements, such as carbon, where the spin--orbit
interaction is small.
\end{itemize}

\section{Collisional processes in plasma}

\begin{figure}[!h]
\centerline{\includegraphics{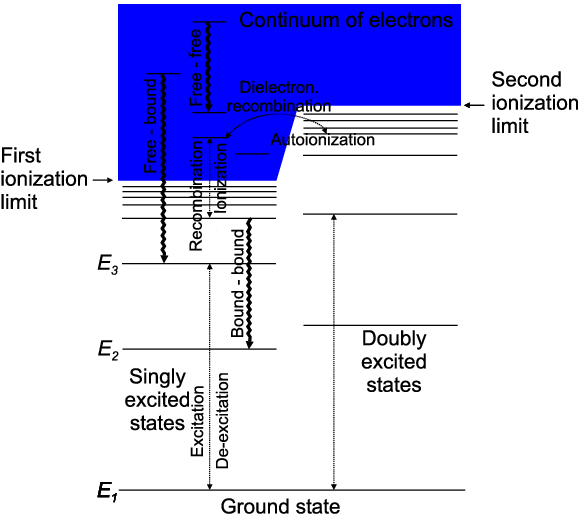}} \captionstyle{hang} \setlength{\captionmargin}{2cm}
\caption{Several possible radiative and collisional processes. \small{(\mbox{Radiative processes are labeled by
wavy line.})}} \label{procesy}
\end{figure}

Similarly to radiative processes, we can distinguish between
collisional excitation -- de-excitation, ionization --
recombination, etc. But on the contrary to radiative processes,
collisional transitions between two states do not follow any
selection rules. The crucial collisional process in a plasma is an
\emph{interaction of a bound electron with free electrons}. The
collision of a bound electron with ions is much more less
significant due to substantial diference in mass. When a free
electron collides with an electron bounded in an ion A, excitation
or ionization of a bound electron can occur \vspace{0.2cm}

\vspace{0.2cm}
\begin{tabular}{l l l l}
 \hspace{1.5cm} A$^z+e^-$ & $\leftrightarrow$ & A$^{z*}+e^-$ &(excitation,
 de-excitation)\\[0.2cm]
 \hspace{1.5cm}  A$^z+e^-$ & $\leftrightarrow$ & A$^{z+1}+e^-+e^-$ &(ionization, three-body
 recombination) \\
\end{tabular}

\vspace{0.3cm} In three-body recombination, the inverse of
collisional ionization, an excited bound state of the ion A$^{z}$
is formed and the excess energy is given to an electron. The
cross--section of this reaction is increasing with the square of
the electron density $n_\mathrm{e}$ and is larger for transitions
into highly excited levels. On the contrary to that, the radiative
capture of an electron occurs mainly into the ground state

\vspace{0.2cm}
\begin{tabular}{l l l p{5cm}}
 \hspace{1.52cm} A$^{z+1}+e^-$ & $\rightarrow$ & A$^{z}+h\nu$ &\hspace{0.77cm} (radiative~capture) \\
\end{tabular}

\vspace{0.3cm} In case of high--temperature and low density plasma
($n_\mathrm{e}<10^{16}\,\mathrm{cm}^{-3}$), the dominant
recombination process is dielectronic recombination: a free
electron is resonantly captured in a high level, with simultaneous
excitation of one of the electrons of the recombining ion
A$^{z+1}$. A doubly--excited ion A$^{z**}$ is formed

\vspace{0.2cm}
\begin{tabular}{l l l l}
\hspace{1.5cm} A$^{z+1}+e^-$ & $\leftrightarrow$ & A$^{z**}$
&\hspace{1.3cm} (dielectronic recombination, autoionization)
\end{tabular}

\vspace{0.3cm} As the doubly--excited state is above the
ionization limit of the recombined ion it is unstable. The two
electron excited state can either undergo the inversion process
--- autoionization or radiatively decay by the emission of photons.

Finally we mention the charge--exchange recombination that happens
during collision between two ions or between ion and atom. When
the charge of ion A is greater than that of ion B, the electron
bounded in ion A could be captured by the other ion B into a
highly excited level

\vspace{0.2cm}
\begin{tabular}{l l l l}
\hspace{1.5cm} A$^{z_\mathrm{A}}+B^{z_\mathrm{B}}$ & $\rightarrow$
& A$^{z_\mathrm{A}-1}+B^{z_\mathrm{B}+1}$ &(charge--exchange
recombination)
\end{tabular}

\vspace{0.3cm} The quantitative description of collisional
processes begins with the cross--section $\sigma (v)$. The number
of transitions ``a'' (of an ion A induced by electrons) per unit
time and per unit volume is given by equation
\begin{equation}
R_\mathrm{a}=-\frac{\diff n_\mathrm{A}}{\diff t}=\langle\sigma
(v)\cdot v\rangle
n_\mathrm{e}n_\mathrm{A}=C_\mathrm{a}n_\mathrm{A}
\end{equation}

where $\langle\sigma (v)\cdot v\rangle=\int\sigma
(v)f_\mathrm{e}(v)v\diff v$ represent so-called rate coefficient.
The rate coefficient is calculated by averaging of $\sigma
(v)\cdot v$ over the electron velocity distribution $f_e(v)$. The
excitation/deexcitation rate coefficient is usually labeled as
$X$, ionization rate coefficient as $S$, and recombination
coefficient as $\alpha$. The quantity $C_a$ is called as the
probability of collision of one ion A with electrons.

\section{Population of energy levels}

The rate of radiative and collisional processes in plasma
determine the population of each energy level. In order to
simplify notation, the rate of all collisions filling the upper
level ``u'' will be marked as $R^\mathrm{c}_{\rightarrow
\mathrm{u}}$, similarly the rate of radiative processes will be
marked as $R^\mathrm{r}_{\rightarrow \mathrm{u}}$ and the rate of
collisions depopulating the level ``u'' as
$R^\mathrm{c}_{\mathrm{u}\rightarrow}=C_{\mathrm{u}\rightarrow}n_\mathrm{u}=X_{\mathrm{u}\rightarrow}n_\mathrm{e}n_\mathrm{u}$.
The symbol $A_{\mathrm{u}\rightarrow}$ stands for the total
transition probability for emission from the level ``u''. By using
these quantities we can write the following rate equation
\begin{equation}
\label{rychlostnirovnice} \frac{\diff n_\mathrm{u}}{\diff
t}=R^\mathrm{c}_{\rightarrow \mathrm{u}}+R^\mathrm{r}_{\rightarrow
\mathrm{u}}-R^\mathrm{c}_{\mathrm{u}\rightarrow}-A_{\mathrm{u}\rightarrow}n_\mathrm{u}
\end{equation}

Usually $n_\mathrm{e}$ and $T_\mathrm{e}$ change slowly compared
to atomic time constants
$\tau_\mathrm{u}=1/(A_{\mathrm{u}\rightarrow}+C_{\mathrm{u}\rightarrow})$.
It means that the the population density $n_\mathrm{u}$ could be
assumed to be in quasi--equilibrium where $\diff n_u/\diff t$.
Simplifying the rate equation~\ref{rychlostnirovnice} we obtain
the population of upper level in collisional--radiative
equilibrium
\begin{equation}
\label{quasiequilibrium}
 n_\mathrm{u}=\frac{R^\mathrm{c}_{\rightarrow
\mathrm{u}}+R^\mathrm{r}_{\rightarrow
\mathrm{u}}}{A_{\mathrm{u}\rightarrow}+C_{\mathrm{u}\rightarrow}}
\end{equation}

The analytic solution of any model taking into account all
processes is still too complicated and it is necessary to use
numerical simulation (For our purposes we used time--dependent
atomic physics code FLY described in appendix~\ref{appendixFLY}).
However, simplifications of equation~\ref{quasiequilibrium} are
still possible in two limiting cases. In case of low density
plasma with $n_\mathrm{e}<10^{14}$~cm$^{-3}$ the population
follows the corona model. In the following we will restrict to the
other limiting case, to high density plasma in LTE (Local
Thermodynamic Equilibrium).

\section{Local thermodynamic equilibrium}

The criterion for LTE is that the collisional rates must be much
larger that radiative rates. Then the radiative terms in equation
\ref{quasiequilibrium} can be neglected and we get
\begin{equation}
\label{LTE1}
 n_\mathrm{u}=\frac{R^\mathrm{c}_{\rightarrow
\mathrm{u}}}{C_{\mathrm{u}\rightarrow}}=\frac{n_\mathrm{e}X_{\rightarrow
\mathrm{u}}}{X_{\mathrm{u}\rightarrow}}
\end{equation}

From the principle of the detailed balance\footnote{Every process
must be balanced by its exact inverse.} follows that
\begin{equation}
\label{LTE2} \frac{X_{\mathrm{l}\rightarrow
\mathrm{u}}}{X_{\mathrm{u}\rightarrow\mathrm{l}}}=\frac{g_\mathrm{u}}{g_\mathrm{l}}\mathrm{e}^{-\frac{E_\mathrm{u}-E_\mathrm{l}}{kT_\mathrm{e}}}
\end{equation}

where $g_\mathrm{u}$, $g_\mathrm{l}$ are the statistical weights
for levels with energies $E_\mathrm{u}$ and $E_\mathrm{l}$,
respectively. Applying equation \ref{LTE2} to any two levels in
atomic species and combining it with equation~\ref{LTE1} it is
possible to derive the well--known Boltzmann distribution for the
level population densities
\begin{equation}
\frac{n_\mathrm{u}}{n_\mathrm{l}}=\frac{g_\mathrm{u}}{g_\mathrm{l}}\cdot
e^{-\frac{E_\mathrm{{u}}-E_\mathrm{{l}}}{kT_\mathrm{e}}}=\frac{g_\mathrm{u}}{g_\mathrm{l}}\cdot
e^{-\frac{h\nu}{kT_\mathrm{e}}} \label{Boltzmann}
\end{equation}

Local thermodynamic equilibrium represents the equilibrium between
particles. The velocities of ions and electrons are described by a
Maxwell distribution. Temperature $T_\mathrm{e}$ may vary from one
place to another, hence the name ``local''. The population density
is described by Boltzmann equation~\ref{Boltzmann} with a
temperature identical with that for the electron velocity
distribution. When we extend Boltzmann relation to continuum
states~\cite{Griem97} we can arrive the Saha equation
\begin{eqnarray}
\frac{n_\mathrm{e}n^{z+1}}{n^z}&=&2\frac{Q^{z+1}(T_\mathrm{e})}{Q^z(T_\mathrm{e})}
\left( \frac{2\pi
m_\mathrm{e}kT_\mathrm{e}}{h^{2}}\right)^{3/2} \mathrm{e}^{-\frac{E_{i}}{kT_\mathrm{e}}} \nonumber\\
\frac{n_\mathrm{e}n^{z+1}}{n^z}&=&6.10^{21}\frac{Q^{z+1}(T_\mathrm{e})}{Q^z(T_\mathrm{e})}T_\mathrm{e}^{3/2}\mathrm{e}^{-\frac{E_i}{T_\mathrm{e}}}\quad[\mathrm{eV;}\,\mathrm{cm}^{-3}]
\label{Saha}
\end{eqnarray}

that describes the total densities of adjacent ionization stages
$n^z$ and $n^{z+1}$. The term $+ze$ represents the ion charge.
$E_{i}$ stands for ionizing energy of an ion/atom with the density
$n^z$. $Q(T_e)$ is the partition function defined by
\begin{equation}
Q^z(T_\mathrm{e})=\sum_ig_i^z\cdot
\mathrm{e}^{-\frac{E_i-E_1}{kT_\mathrm{e}}}
\end{equation}

The sum goes over all bounded states $i$. The number of terms that
are included to evaluate the partition function depends not only
on the plasma temperature but also on the density.

The thermodynamic equilibrium is further described by the Planck
blackbody function for radiation energy with the same temperature
$T=T_\mathrm{e}$. This is no more valid in LTE where the radiation
density could be below the blackbody level.

\section{Validity conditions for local thermodynamic equilibrium}

The first necessary condition of LTE is a Maxwell distribution of
electron velocities.

Another condition is given by the validity of reducing
equation~\ref{quasiequilibrium} to equation~\ref{LTE1}. It means
that the unequality  $A_{u\rightarrow}\ll C_{u\rightarrow}$ has to
be satisfied. Usually a factor of ten is considered as
sufficiently high, i.e. $10\ A_{u\rightarrow}\leq
C_{u\rightarrow}$. Unfortunately it is impossible to derive any
easy criterion for \emph{complete} LTE (i.e. for the populations
of all levels). The review of C.~De~Michelis and M.~Mattioli
provides the necessary, but not sufficient,
criterion~\cite{deMichelis81}
\begin{equation}
n_\mathrm{e}\geq 1,8.10^{14}\sqrt{kT_\mathrm{e}}\Delta
E^3_\mathrm{ul} \quad [\mathrm{eV; cm}^{-3}]
\end{equation}

This criterion is difficult to satisfy especially for the largest
energy level difference $\Delta E_\mathrm{ul}$ in the level
scheme. Nevertheless, for any $n_\mathrm{e}$ the collisions still
dominate between high--lying levels. Level, above which excited
stated are in equilibrium with the ground state of the next
ionization stage, is called thermal limit. Then we said that
plasma is in \emph{partial} LTE. We use the following
criterion~\cite{Griem64}
\begin{equation}
n_\mathrm{e}\geq
7.10^{17}\frac{(z+1)^6}{n_{th}^{17/2}}\sqrt{\frac{kT_\mathrm{e}}{E_\mathrm{H}}}
\quad [\mathrm{eV; cm}^{-3}]
\end{equation}

that determines the minimal electron density $n_\mathrm{e}$ which
is needed for partial LTE of levels above the principal number
$n_\mathrm{TH}$. Here $z$~is the effective nuclear charge and
$E_\mathrm{H}\doteq13,6$ eV is the ionization energy of hydrogen.

Finally we can mention the importance of the relaxation time. It
is evident that the time necessary for making an equilibrium must
be substantially smaller than the characteristic time of processes
in plasma. More details about the conditions can be found
in~\cite{Griem64,Griem97,Thorne99}.

\section{Radiative transfer}

Until then we were interested in the influence of collisional and
radiative processes on the population of energy levels. It was
important since the population of energy level $n_\mathrm{u}$ and
the transition probability of spontaneous emission determines the
local emission in the plasma. The local emission is described by
the emissivity, the power emitted per unit solid angle per Hz by
unit volume
\begin{equation}
\epsilon_\nu=\frac{\diff^3 \Phi}{\diff V\diff \Omega\diff \nu}
\end{equation}

and
\begin{equation}
\epsilon_\nu(\mathrm{u}\rightarrow
\mathrm{l})=\frac{h\nu}{4\pi}A_{\mathrm{ul}}n_\mathrm{u}
\end{equation}

The importance of emissivity lies in the fact that it contains
information about local properties of the plasma. However, it is
impossible to directly determine the emissivity by passive
emission spectroscopy. We usually measured the spectral radiance
$L_\nu$ at the surface of plasma, the power emitted per unit solid
angle per Hz by unit projected area
\begin{equation}
L_\nu=\frac{\diff^3 \Phi}{\diff S \cos\theta \diff \Omega\diff
\nu}
\end{equation}

 The relation between these two quantities is trivial
only in case of optically thin plasma where the absorption and
re-emission of photons are neglected. Otherwise we have to solve
the equation of radiative transport, which may be written for the
line of sight along the axis $X$
\begin{equation}
\label{radiativetransfer} \diff L_{\nu}(\vec{r},\Omega)=\bigg[
\epsilon_{\nu}(\vec{r},\Omega)-\kappa(\nu,\vec{r})
L_{\nu}(\vec{r},\Omega)\bigg] \diff x
\end{equation}

Here $\kappa(\nu,\vec{r})$ represents the effective absorption
coefficient that could be negative if stimulated emission occurs.
We now define a quantity called the source function
$S_{\nu}(\vec{r})$ as the ratio of the emissivity to the
absorption coefficient
\begin{equation}
 S_{\nu}(\vec{r},\Omega)=\frac{\epsilon_{\nu}(\vec{r},\Omega)}{\kappa(\nu,\vec{r})}
\end{equation}

And by using the optical depth $\tau(\nu,\vec{r})$
\begin{equation}
\diff \tau(\nu,\vec{r})=\kappa(\nu,\vec{r})\diff x
\end{equation}

we can rewrite equation \ref{radiativetransfer} as follows
\begin{equation}
\frac{\diff L_{\nu}(\vec{r},\Omega)}{\diff
\tau(\nu,\vec{r})}=S_{\nu}(\vec{r},\Omega)-L_{\nu}(\vec{r},\Omega)
\end{equation}

Unfortunatelly this equation cannot be solved in general
(cf.~\cite{Aschke00, Kunze02}) because the emissivity and
absorption coefficient may have different spectral dependence.
Moreover, the absorption of photons influences the population of
energy levels and thus it is necessary to solve the equation
\ref{radiativetransfer} together with the system of
equations~\ref{rychlostnirovnice}.

The solution of equation~\ref{radiativetransfer} can be found only
in limiting cases. If we suppose the homogenous plasma with the
characteristic length along the line of sight $l_\Omega$ and the
spatially isotropic source function $S_{\nu}$ we can arrive at the
relation
\begin{equation}
L_{\nu}=S_{\nu}(1-\mathrm{e}^{-\tau(\nu)})
\end{equation}

where $\tau(\nu)=\int\diff \tau(\nu,\vec{r})=\kappa(\nu)
l_\Omega$.

Furthermore, if the plasma is optically thin \mbox{($\tau\ll 1$)},
i.e. without absorption,  we can use the Taylor series
$\mathrm{e}^{-\tau(\nu)}\approx 1-\tau(\nu)$. Then we obtain
\begin{equation}
L_{\nu}\approx\int\epsilon_{\nu}(\vec{r},\Omega)\diff
x=\epsilon_{\nu}l_\Omega
\end{equation}

In another limiting case $\tau\gg 1$, we can derive
\begin{equation}
L_{\nu}=S_{\nu}=\frac{\epsilon_{\nu}}{\kappa(\nu)}=\frac{2h\nu^3}{c^2}\cdot\frac{1}{e^{h\nu/kT}-1}
\end{equation}

The last equality is valid in case of the plasma in thermodynamic
equilibrium. The limiting case $\tau\gg 1$ is not reached in the
entire spectral range. Since the absorption increases with
$\lambda^2$, the plasma becomes optically thick towards long
wavelength~\cite{Kunze89}. The emission lines become optically
thick more easily than continuum at short wavelengths. From the
experimental point of view it is necessary to know if the spectral
line is optically thick. For Doppler--broadened lines and the
plasma in LTE, the optical thickness at the line centre
$\nu_0=c/\lambda_0$ is given by
\begin{equation}
\tau(\nu_0)=r_\mathrm{B}\sqrt{\frac{\pi M_\mathrm{i}c^2}{2kT}
}\lambda_0f_{\mathrm{ul}}n_\mathrm{l} l_\Omega
\end{equation}

where $r_\mathrm{B}=e^2/4\pi\varepsilon_0m_\mathrm{e}c^2$ is the
classical (Bohr) electron radius. Substituting known constants in
the previous equation, we get the equation
\begin{equation}
\tau(\nu_0)\doteq1,08.10^{19}\sqrt{\frac{M_\mathrm{i}}{2kT}}
\lambda_0f_{ul}n_l l_\Omega
\end{equation}

Here the ion mass $M_\mathrm{i}$ is in atomic units
$m_\mathrm{u}$, temperature $kT$ in~eV, the population of lower
level $n_\mathrm{l}$ in~m$^{3}$, the wavelength $\lambda_0$ in~nm,
and the length of plasma $l_\Omega$ in~m.

Experimentally we can check if the emission lines are optically
thick or thin by comparing the relative intensities of close
multiplet lines. The radiance ratio of two optically thin
multiplet lines is determined by the statistical weights of lower
levels $g_\mathrm{l}$ and the oscillator strengths $f_\mathrm{lu}$
\begin{equation}
\frac{L_{\nu_1}}{L_{\nu_2}}=\frac{f_{\mathrm{l}_1\mathrm{u}_1}g_{\mathrm{l}_1}}{f_{\mathrm{l}_1\mathrm{u}_2}g_{\mathrm{l}_2}}
\end{equation}

If the measured ratio is higher in favor of the weaker line, the
spectral lines are not optically thin. As a result the temperature
cannot be easily determine by the intensity ratio of spectral
lines.

\section{Intensity of spectral lines}

The intensity of spectral line $I$ is often refereed in the
scientific literature. The fact of the matter is that the correct
term is the spectral radiance $L_\nu$, mostly spatially and/or
temporally integrated. As the intensity became common we will use
it in the following text in spite of that the spectral radiance is
more appropriate.

\section{Spectroscopic measurements of plasma parameters}

The emission spectroscopy of plasma belongs to one of the
fundamental passive diagnostic technique. The emissivity of plasma
contains a lot of information about plasma properties and
dynamics. The key issue is the choice of a suitable method which
enabled the estimation of plasma parameters, especially the
electron temperature and density. Our choice of a method was
predetermined by the properties of our grating spectrograph (see
subsection~\ref{spectrograph} on page~\pageref{spectrograph}). It
enables only the measurement of relative intensities of spectral
lines. The measurement of line profile was not possible due to
limited spectral resolution. That is why the manifold choice of
spectroscopic technique (cf. \cite{Griem64, Griem97,
deMichelis81}) reduces to several fundamental methods.

\section{Spectroscopic measurement of temperature and density}

First, it is important to remember that a spectroscopic
measurement of temperature is actually measurement of a parameter
determining some equilibrium distribution \cite{Thorne99}.
Therefore we can distinguish between the electron temperature
$T_\mathrm{e}$ and the ion temperature $T_\mathrm{i}$. Moreover we
can distinguish between the electron temperature occurring in the
Maxwell velocity distribution, in the Boltzmann
distribution~\ref{Boltzmann} (so-called population or excitation
temperature), in the Saha--Boltzmann equation~\ref{Saha}
(ionization temperature), and etc. Unless any equilibrium
distribution exists, the temperature is not defined and the plasma
have to be described by the distribution functions. Most of
spectroscopic temperature measurement primarily yield
$T_\mathrm{e}$. The same was in our case. The kind of the electron
temperature (excitation, ionization, etc.) follows from the method
used and will not be specified in our work.

\begin{itemize}
\item[--] Very easy and undemanding method of the rough
temperature measurement is the identification of ionic states in a
plasma. In order ro reach an ionic state with ionization potential
$E_\mathrm{i}$, the electron temperature must obey
\begin{equation}
\label{odhadteploty}
 T_\mathrm{e}>C_\mathrm{i} E_\mathrm{i}
\end{equation}

with $C_\mathrm{i}$ varying approximately between 0.1 and 0.3
\cite{Hauer91}.

More accurate value of temperature can be obtain from the
calculation of ionization equilibrium (the temperature dependence
of population of various ionic states). The free parameter in this
calculation is the electron or ion density. To calculate
ionization equilibrium we used atomic physics code FLY.

\item[--] Another common method is based on relative line
intensities of the same ion.

Provided the plasma is in LTE or at least in partial LTE, the
population of energy levels follows the Bolzmann
distribution~\ref{Boltzmann}. Then the ratio of two optically thin
spectral lines is given by
\begin{equation}
\label{ratio}
\frac{L_{\nu}}{L_{\nu'}}=\frac{A_\mathrm{ul}g_\mathrm{u}\lambda '}
{A_\mathrm{u'l'}g_\mathrm{u'}\lambda}\cdot
\mathrm{e}^{-(E_\mathrm{u}-E_\mathrm{u'})/kT_\mathrm{e}}
\end{equation}

It can be clearly seen from Eq.~\ref{ratio} that, besides several
constants, the ratio is dependent only the electron temperature.
The sufficient sensitivity is achieved for
$E_\mathrm{u}-E_\mathrm{u'}> kT_\mathrm{e}$. This method can be
extended to more spectral lines than two. We can make a graph with
$\ln (L_{\nu} \lambda/g_\mathrm{u} A_\mathrm{ul})$ on the
$x$--axis and with the energy of upper level $E_\mathrm{u}$ on the
$y$--axis. The slope of the line then equals $-T_\mathrm{e}$. This
method was used in cases when the code FLY cannot be applied, e.g.
for Be--like ions.

\item[--] In the regions where (partial) LTE approximation is no
more valid, the ratio of two spectral lines is not only
temperature-- but also density--dependent. In such circumstances a
detailed accounting must be made of the ionization, recombination,
excitation, deexcitation and radiative transfer. As far as this
work is concerned, we used the code FLY to calculate the
population of the states and the ratio of line intensities in
non--LTE approximation (usually in collisional--radiative
equilibrium). The suite FLY enables also the reconstruction of the
synthetic spectrum for a particular temperature and density. Since
the ratio of spectral lines is not only temperature dependent we
can estimate the density. It was very useful since the other
methods of density measurement (such as Stark broadening,
depression of ionization potential, Inglis--Teller limit, or the
ratio of resonance and intercombination lines of He--like ions)
cannot be applied.
\end{itemize}

\chapter{Code FLY}
\label{appendixFLY}

\section{Basic parameters}
\pagenumbering{Roman}

FLY~\cite{Lee96,Lee95} is a commercially available suite of
computer codes which was developed for designing and/or analyzing
experiments where $K$--shell spectra\footnote{$K$--shell
spectroscopy is engaged in the radiative transitions to the most
inner shell ($K$--shell) of ions.} are observed. The FLY suite is
capable of simulating $K$--shell emitters with the atomic number
$Z$ from 2 to 26, i.e., from helium to iron. The suite allows the
user to calculate the population of the states in an LTE or
non--LTE approximation, by assuming steady--state or a time
dependent evolution. The kinetics model FLY provides details of
the level populations of hydrogen--, helium-- and lithium--like
ions. Less ionized species are represented as a ground state only.
FLY is a "zero--dimension" suite of codes, thus the plasma is
specified with the local conditions. The optical depth effects are
approximated for a homogenous plasma "column" only. The most
important characteristics of the suite can be summarized in the
following items:

\begin{itemize}
\item $0$-dimension post-processing of MHD. \item Atomic number
$Z$ from 2 to 26, i.e., from helium to iron. \item K--shell
spectroscopy: detailed information on H-, He- a Li- like ion
stages. $K$-shell satellite lines and also continuum radiation are
included. \item Steady-state (either LTE, or non-LTE) as well as
time--dependent solution of rate equations.
 \item Line profile synthesis --- Doppler profile. Stark broadening
for specific transition only. \item Effect of optical depth within
the escape factor approximation \item External radiation field is
possible to include. \item Easy of use. Comparison of the
synthetic spectrum with the experimental one.
\end{itemize}

\section{Description}

The suite of code consisted of three parts\ -- FLY, FLYPAPER and
FLYSPEC codes.

\section{FLY}
The first code in the suite, FLY, calculates the level populations
of hydrogen--, helium-- and lithium--like ions. The population of
energy levels can be solved either in non--LTE or LTE case. The
rate equations for populations include the most relevant ionizing,
recombining, exciting and deexciting processes. The necessary
input is the atomic number of interest together with the history
of magnetohydrodynamic parameters. The other possible input is the
grid of temperature and density for which the populations will be
calculated. When the time history of plasma parameters is known,
the code calculates a time-dependent evolution of the populations.
When a grid of temperatures and densities is input, the code
computes a steady state approximation of population levels. The
output file of the FLY code serves as an input into the other two
codes of the suite --- FLYPAPER and FLYSPEC.

\section{FLYPAPER}

FLYPAPER code can be used to evaluate:

\begin{itemize}
\item populations of levels, \item the ratio of line intensities,
\item optical depth
\end{itemize}

as a function of the time or plasma parameters (density and
temperature).

\section{FLYSPEC}
FLYSPEC code allows the reconstruction of the synthetic spectrum
for a particular time or for one temperature and density. The line
profiles can be calculated for certain transitions: the Lyman and
Balmer series for hydrogen--like ions, $1s^{2}$ $^{1}S_{0}$ --
$1snp$ $^{1}P$ transitions for helium--like ions, and transitions
to the ground levels $2s,2p$ in the case of lithium--like ions.
The recombination emission is calculated for mentioned series
only. In addition the user can perform integrations of spectra
over time.

\section{Code limitation}
Firstly, it should be stressed that the FLY suite is a
$0$--dimension code. Therefore a correct treatment of radiative
transfer (which is non--local problem especially where a density
gradient occurs) is not possible. Moreover, only Doppler
broadening is incorporated in FLY code and therefore the optical
depth effects are overestimated.

Secondly, if we need to obtain synthetic spectra of $L$-- or $M$--
shell emitters we also need to use another code than FLY. This is
true also for detail description of Li--like ionization state
because lower excited state (Be--like) is described only by a
single ground state\footnote{This restriction was overcome in
FLYCHK, the extension of FLY~\cite{Chung03}.}. Since FLYSPEC code
includes recombination for certain transition only, the continuum
spectrum is underestimated.

Thirdly, the appropriate use of the post--processor assumes that
the preceding MHD modelling of plasma evolution is not influenced
by the fact that the detail radiative processes are not included.
This condition need not be fulfilled in strongly radiating plasma
consisting from high $Z$ elements.

Fourthly, another serious problem represents non--Maxwellian
distribution of electrons since it often occurs allong $Z$--axis
in $Z$--pinch plasma and can not be described by means of electron
temperature.

And lastly we can say that FLYSPEC provide instrumental broading
that was not sufficient. Therefore we have to process the
synthetic spectra with spreadsheet program in order to compare
them with the experimental ones.

\section{Platform}
The kernel of the suite FLY was written in FORTRAN77 language.
Running the code does not require any atomic and spectroscopic
data since they are internally included. Programme runs on any
UNIX/Linux workstation as well as on desktop PC under MS-DOS.

More details can be found in ref. \cite{Lee96, Lee95}.
